# Supplementary material for: SVRG Meets AdaGrad: Painless Variance Reduction
Source: arXiv:2102.09645 source file (2021-11-03)
Supplement: Supplementary file 1 [file Additional-algorithms.tex]

\section{Algorithms}
\label{app:add-algorithms}
\vspace{-3ex}
\begin{algorithm}[H]
\caption{\adasvrg/ with adaptive termination test}
\label{alg:adasvrg-at-test}
\textbf{Input}: $w_0$ (initial point), $K$ (outer-loops), $\theta$ (adaptive termination parameter), $M$ (maximum inner-loops) \\
\For{$k \leftarrow 0$  \KwTo  $K-1$}{
    Compute full gradient $\nabla f(w_k)$ \\
    $\eta_k \leftarrow$ Compute step-size \\
    Initialize \adagrad/: $x_1 = w_k$ and $G_0 = \mathbf{0}$ \\
    \For{$t \leftarrow 1$ \KwTo $M$}{
    Sample $i_t \sim \text{Uniform}\{1, 2, \ldots n\}$ \\
    $g_t = \nabla \fit(x_t) - \nabla \fit(w_k) + \nabla f(w_k)$\\
    $G_t = \begin{cases}G_{t-1} + g_t g_t^\top &\text{(full matrix version)} \\
    G_{t-1} + \text{diag}(g_t g_t^\top) &\text{(diagonal version)}\\
    G_{t-1} + g_t^\top g_t&\text{(scalar version)} 
    \end{cases} $\\
    $A_t = G_t^{1/2}$\\
    \If{$t$ mod $2$ $==0$ and $t \geq n$}
    {$R = \frac{\|G_{t}\|^2_* - \|G_{t/2}\|^2_*}{\|G_{t/2}\|^2_*}$\\
    \If{$R \geq \theta$}{
    Terminate inner loop
    }
    }
    $x_{t+1} = \proj{X, A_t}{x_t - \eta_{k} A_t^{-1}g_t}$
    }
    $w_{k+1} = \frac{1}{m_k} \sum_{t=1}^{m_k} x_t$
}
Return $w_{K}$
\end{algorithm}

% \begin{algorithm}[H]
% \caption{Hybrid \adagrad/-\adasvrg/}
% \label{alg:hybrid}
% \textbf{Input}: $x_1$ (initial point), $T$ (iteration budget), $M$ (maximum inner loops), $\theta$ (adaptive termination parameter) \\
% \textbf{Phase 1: \adagrad/} \\
%     $G_0 \leftarrow \mathbf{0}$ \\
%     \For{$t \leftarrow 1$ \KwTo $T$}{
%     Sample $i_t \sim \text{Uniform}\{1, 2, \ldots n\}$ \\
%     $\eta_t \leftarrow$ Compute step-size \\
%     $g_t = \nabla \fit(x_t)$ \\
%     $G_t = \begin{cases}G_{t-1} + g_t g_t^\top &\text{(full matrix version)} \\
%     G_{t-1} + \text{diag}(g_t g_t^\top) &\text{(diagonal version)}\\
%     G_{t-1} + g_t^\top g_t&\text{(scalar version)} 
%     \end{cases} $\\
%     $A_t = G_t^{1/2}$\\
%     \If{$t$ mod $2$ $==0$ and $t \geq 2n$}
%     {$R = \frac{\|G_{t}\|^2_* - \|G_{t/2}\|^2_*}{\|G_{t/2}\|^2_*}$\\
%     \If{$R \geq \theta$}{
%     $w_0 = x_t$\\
%     Terminate and switch to AdaSVRG
%     }
%     }
%     $x_{t+1} = \proj{X, A_t}{x_t - \eta_{k} A_t^{-1}g_t}$
%     }
%     \textbf{Phase 2: \adasvrg/} \\
%     $K = \floor{\frac{T - t}{n}}$ \\
%     $w_{K}$ = \cref{alg:adasvrg-at-test}($K$, $\theta$, $M$, $w_0$) \\
% Return $w_{K}$
% \end{algorithm}
